# Supplementary material for: Vapor Phase Assembly of Molecular Emitter Crystals for Photonic Integrated Circuits
Source: arXiv:2602.18517 source file (2026-02-19)

DBT Fluorescence

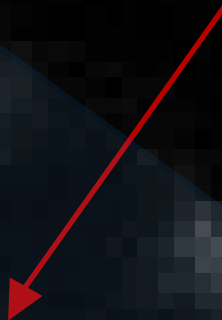

AC

Substrate

10 $\mu$ m

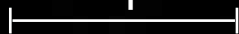

DBT Fluorescence

AC

Substrate

10 $\mu$ m

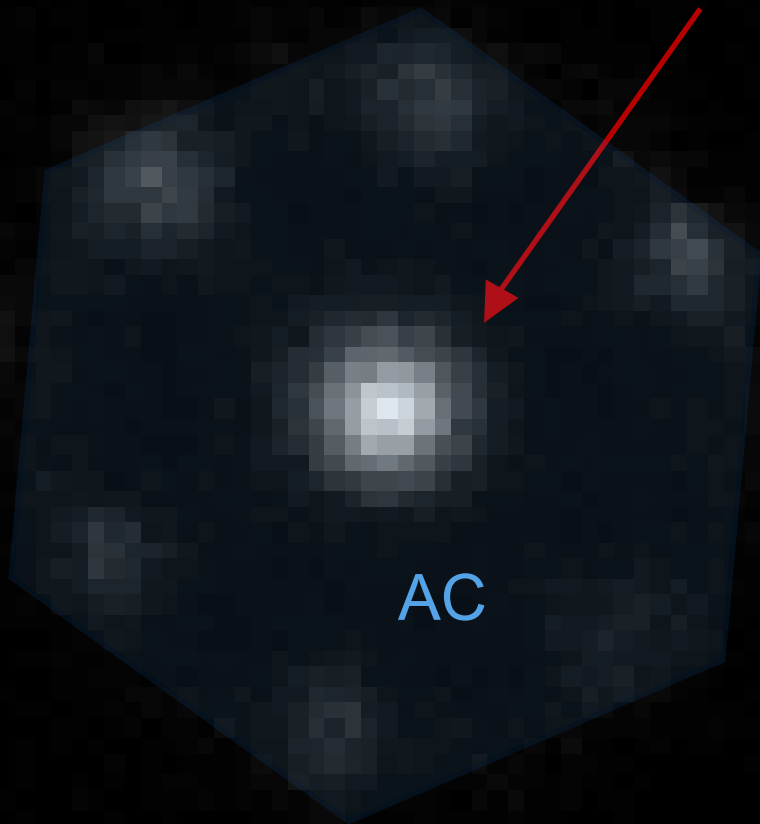

Supplement: Supplementary file 1 [file sm_4.pdf]
